# Supplementary material for: Generating Entangled Steady States in Multistable Open Quantum Systems via Initial State Control
Source: arXiv:2510.07628 source file (2026-02-02)

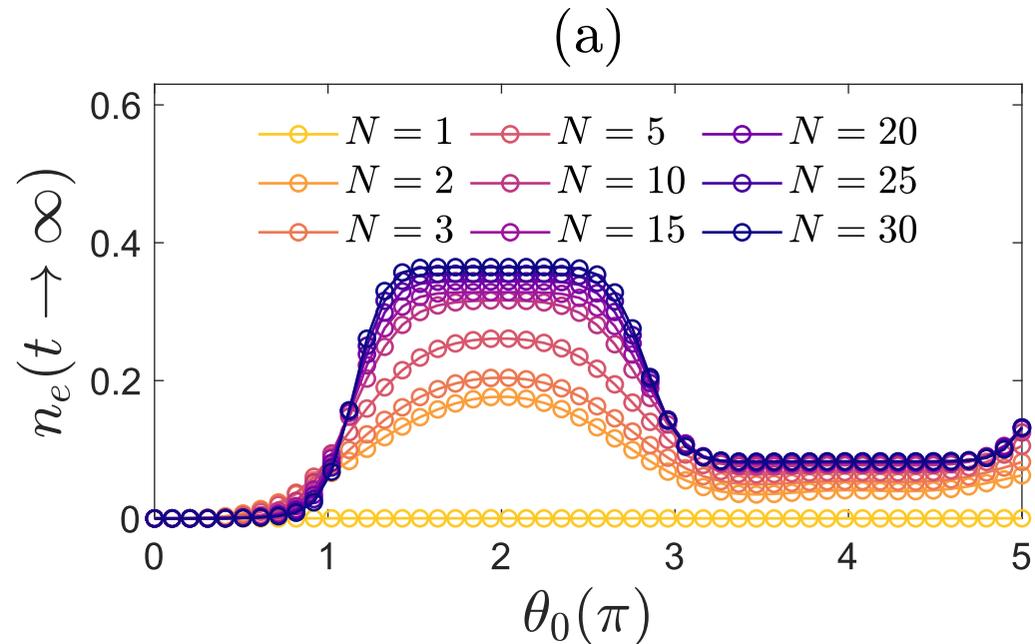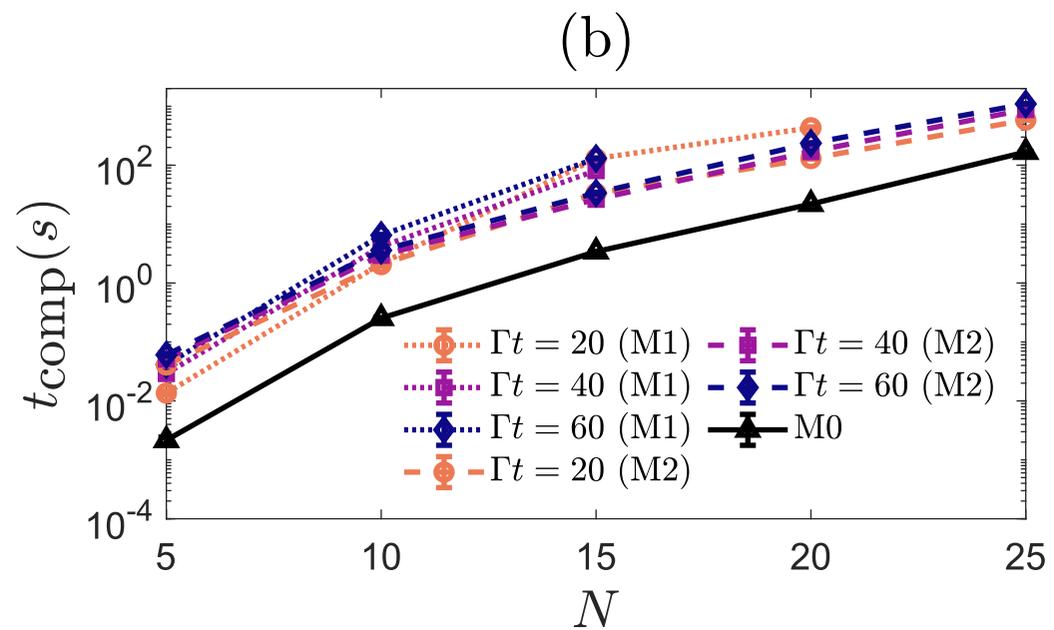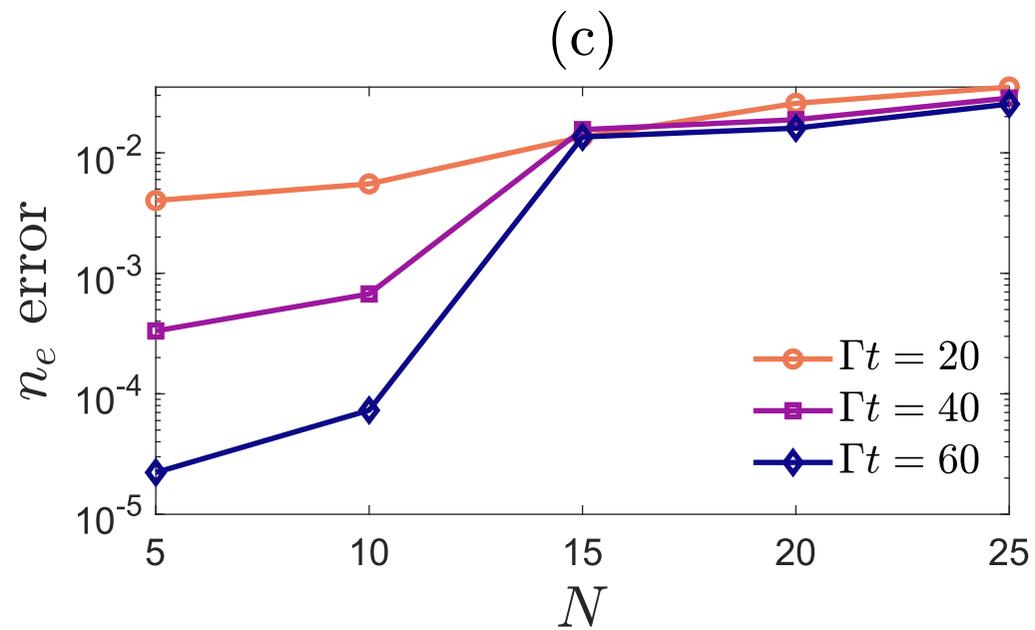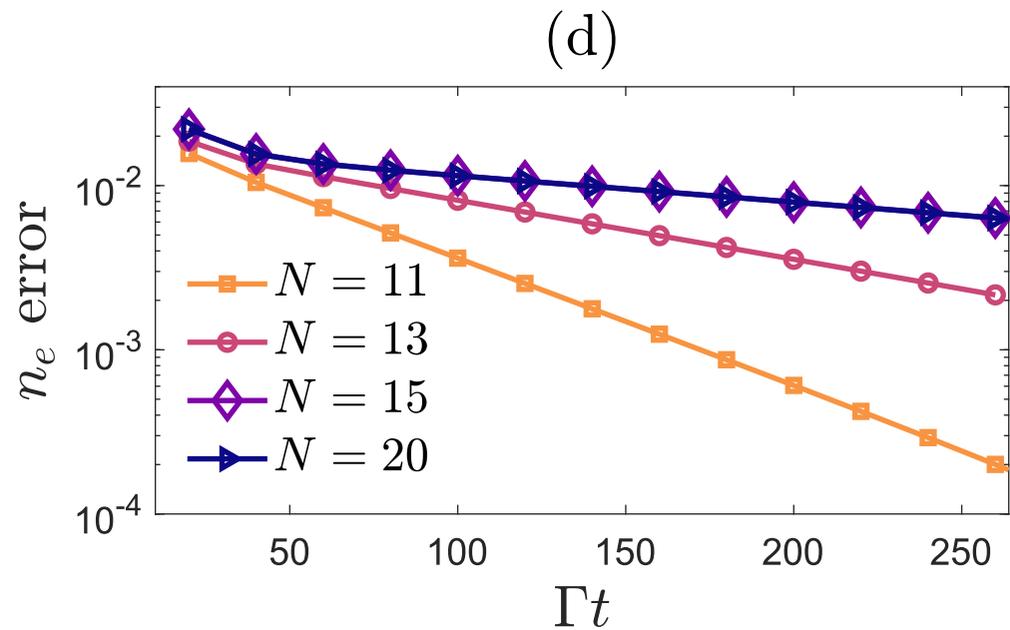

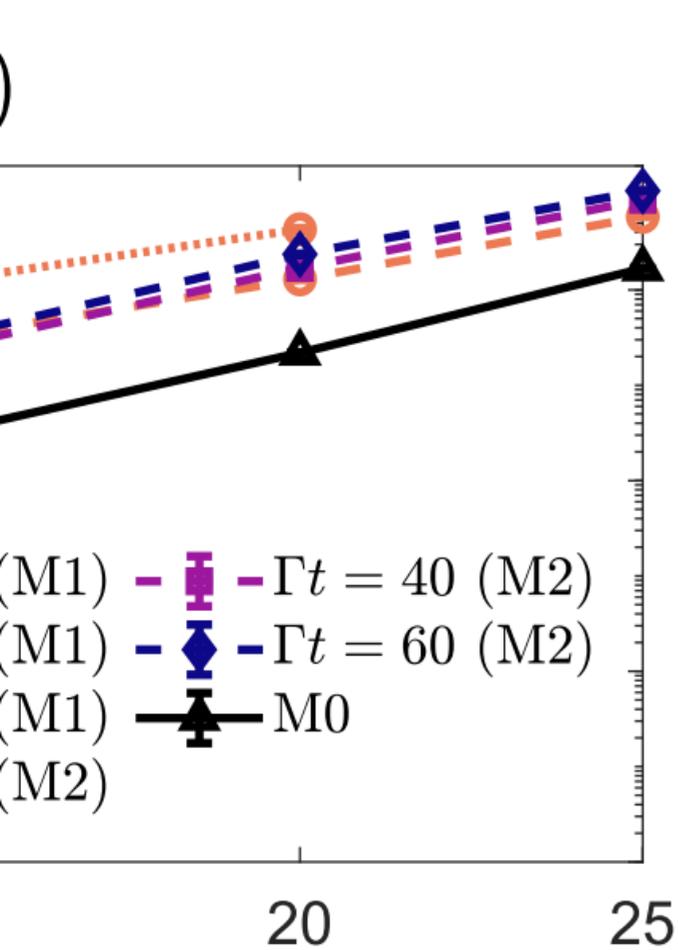

Supplement: Supplementary file 2 [file Fig3Supp.pdf]
